# Supplementary material for: A System-Level Dynamic Binary Translator using Automatically-Learned Translation Rules
Source: arXiv:2402.09688 source file (2024-02-15)
Supplement: Supplementary file 1 [file Appendix.tex]

\appendix
\section{Artifact Appendix}

%%%%%%%%%%%%%%%%%%%%%%%%%%%%%%%%%%%%%%%%%%%%%%%%%%%%%%%%%%%%%%%%%%%%%
\subsection{Abstract}

This artifact includes the executable files, testing scripts and analysis scripts to reproduce all results in Section~\ref{sec:evaluation}.

\subsection{Artifact check-list (meta-information)}

{\small
\begin{itemize}
  \item {\bf Algorithm:} {\em Coordination overhead reduction, coordination elimination, instruction scheduling}
  \item {\bf Program:} Included and compiled SPEC CPU 2006
  \item {\bf Compilation:} No
  \item {\bf Binary:} C executables
  \item {\bf Run-time environment:} Ubuntu 18.04.4 LTS with Linux 3.10.0
  \item {\bf Hardware:} At least 12 threads of CPU and at least 20GB of DRAM
  \item {\bf Metrics:} Speed up, host instructions per guest instruction, dynamic coverage, etc
  \item {\bf Output:} Log files
  \item {\bf Experiments:} Follow the artifact README
  \item {\bf How much disk space required (approximately)?:} More than 20GB
  \item {\bf How much time is needed to prepare workflow (approximately)?:} About 5 minutes
  \item {\bf How much time is needed to complete experiments (approximately)?:} About 6 days
  \item {\bf Publicly available?:} No
\end{itemize}

%%%%%%%%%%%%%%%%%%%%%%%%%%%%%%%%%%%%%%%%%%%%%%%%%%%%%%%%%%%%%%%%%%%%%
\subsection{Description}

\subsubsection{How delivered}

You can download the artifact in Zenodo (https://doi.org/10.5281/zenodo.8256231). It requires 6GB of disk space to unpack the artifact.

\subsubsection{Hardware dependencies}

At least 12 threads of CPU and at least 20GB of DRAM.

\subsubsection{Software dependencies}

The software dependencies are all prepared in the docker image.

%%%%%%%%%%%%%%%%%%%%%%%%%%%%%%%%%%%%%%%%%%%%%%%%%%%%%%%%%%%%%%%%%%%%%
\subsection{Installation}

We use a docker image to pack all of the dependencies as well as binaries of QEMU 6.1 and our enhanced system-level emulator.
Use following commands to load the docker image and start docker containers is enough.

  \$ docker load -i cgo51ae.tar

  \$ docker-compose up -d

%%%%%%%%%%%%%%%%%%%%%%%%%%%%%%%%%%%%%%%%%%%%%%%%%%%%%%%%%%%%%%%%%%%%%
\subsection{Experiment workflow}

% After installation phase, there are two docker containers running.
%b One named "test\_origin" is for QEMU 6.1 and the other named "test\_enhance" is for our enhanced system-level emulator.

To reproduce performance results in Figure~\ref{fig:speedup}, Figure~\ref{fig:opt_speedup}, and Figure~\ref{fig:slowdown}, use {\em start\_p\_origin.sh} to run QEMU 6.1 and use one of the {\em start\_p\_base.sh start\_p\_reduction.sh start\_p\_elimination.sh start\_p\_scheduling.sh} to run the corresponding enhanced version at the same time.
For example, to evaluate the performance of "base" version, run {\em start\_p\_origin.sh} in one console and run {\em start\_p\_base.sh} in another console at the same time.

To reproduce analysis results in Figure~\ref{fig:trans_quality}, Figure~\ref{fig:sync_instr}, and Figure~\ref{fig:coverage}, use {\em start\_a\_origin.sh} and {\em start\_p\_enhance.sh} to run QEMU 6.1 and our full optimized version at the same time.

In other words, the whole experiment workflow consists of 5 executions.
In each execution, run QEMU 6.1 and one of the enhanced versions simultaneously.

%%%%%%%%%%%%%%%%%%%%%%%%%%%%%%%%%%%%%%%%%%%%%%%%%%%%%%%%%%%%%%%%%%%%%
\subsection{Evaluation and expected result}

After each execution, run {\em get.sh} to collect raw data.
Then, for performance raw data, run {\em parse\_p.py} to parse the results.
It will generate a file named "performance.xls" to show the metrics.
For profiling raw data, run {\em parse\_a.py} to parse the results.
It will generate a file named "analysis.xls" to show the metrics.

All results in Section~\ref{sec:evaluation} are expected to be reproduced.

%%%%%%%%%%%%%%%%%%%%%%%%%%%%%%%%%%%%%%%%%%%%%%%%%%%%%%%%%%%%%%%%%%%%%

\subsection{Notes}

Please refer to artifact README for more details and notes.

%%%%%%%%%%%%%%%%%%%%%%%%%%%%%%%%%%%%%%%%%%%%%%%%%%%%%%%%%%%%%%%%%%%%%
